# Supplementary material for: Doc2Spec: Synthesizing Formal Programming Specifications from Natural Language via Grammar Induction
Source: arXiv:2602.04892 source file (2026-10-07)
Supplement: Supplementary file 1 [file 5_rule_formalizer_rust.tex]

\begin{llmex}{LLM Input (Prompt)}

\role{System}
\begin{lstlisting}[style=llmtext]
You can perform the following actions.
Available Actions:
- write_dsl: Return exactly one DSL statement that conforms to the provided grammar for the given rule.
  Input Schema: {
  "type": "object",
  "properties": {
    "dsl": {
      "type": "string",
      "description": "A single DSL statement that ends with ';' and parses with the grammar."
    }
  },
  "required": [
    "dsl"
  ]
}
\end{lstlisting}

\role{User}
\begin{lstlisting}[style=llmtext]



Write ONE DSL statement for the given natural-language rule, using the following Lark grammar.
Rules:
- The DSL must parse with this grammar.
- Do NOT invent predicate names or change arity; only use what appears in the grammar.
- Output exactly one statement and end it with ';'.
- If rule requires certain attributes from the target(provided in JSON format), use JSON path to access them.

Grammar:```
// ===== Base tokens =====
%import common.WS
%import common.ESCAPED_STRING
%import common.SIGNED_NUMBER
%ignore WS

VAR: /[A-Za-z_][A-Za-z0-9_]*/

TRUE: "true"
FALSE: "false"

COMMA: ","

// ===== Target Attribute Selector =====
target_attr_selector: "TargetAttr" LPAREN ESCAPED_STRING RPAREN  // e.g., TargetAttr("<JSONPath>")

// A simple value type used as predicate arguments.
?value: ESCAPED_STRING
      | SIGNED_NUMBER
      | TRUE
      | FALSE
      | VAR
      | target_attr_selector

// ===== DSL entry =====
?start: stmt+

stmt: check (IF condition)? SEMI

IF: "if"
SEMI: ";"

// ===== Condition boolean expression =====
?condition: or_expr

?or_expr: and_expr
       | or_expr OR and_expr   -> or

?and_expr: not_expr
        | and_expr AND not_expr -> and

?not_expr: atom
        | NOT not_expr          -> not

?atom: LPAREN condition RPAREN -> group
     | cond_atom

OR: "or"
AND: "and"
NOT: "not"

LPAREN: "("
RPAREN: ")"

?check: primary_allocatesmemory_0 | primary_returnspointer_1 | primary_mayresultinundefinedbehavior_2 | primary_hasmemoryinitstatus_3 | primary_allocationfailure_4 | primary_implementstrait_5 | primary_legaltraitimplementation_6 | primary_deallocatesmemory_7 | primary_callerguaranteesdeallocatable_8 | primary_allocatedbyallocator_9 | primary_memoryblockdeallocated_10 | primary_mayresultinundefinedbehaviorondealloc_11 | primary_alloczeroedmayresultinundefinedbehavior_12 | primary_alloczeroedreturnsinitialized_13 | primary_resizesmemoryblock_14 | primary_mayresultinundefinedbehavioronpointeraccess_15 | primary_callersatisfiesreallocrequirements_16 | primary_newsizeispositive_17 | primary_roundupsizetoalignment_18 | primary_mayresultinundefinedbehavioronrealloc_19 | primary_allocatorcanallocate_20

primary_allocatesmemory_0: "AllocatesMemory" LPAREN value COMMA value COMMA value RPAREN  // - AllocatesMemory(allocator: Allocator, layout: Layout, memory: Memory): An allocator allocates a memory region that satisfies the specifications of a given layout.
primary_returnspointer_1: "ReturnsPointer" LPAREN value COMMA value COMMA value RPAREN  // - ReturnsPointer(allocator: Allocator, layout: Layout, pointer: Pointer): The allocator returns a pointer as the result of the allocation request for a given layout.
primary_mayresultinundefinedbehavior_2: "MayResultInUndefinedBehavior" LPAREN value COMMA value COMMA value RPAREN  // - MayResultInUndefinedBehavior(allocator: Allocator, layout: Layout, behavior: UndefinedBehavior): Expresses that attempting to allocate memory with a given allocator and layout may lead to undefined behaviour.
primary_hasmemoryinitstatus_3: "HasMemoryInitStatus" LPAREN value COMMA value RPAREN  // - HasMemoryInitStatus(memory: Memory, status: MemoryInit): Associates a memory block with its initialization status, which can be either initialized or uninitialized.
primary_allocationfailure_4: "AllocationFailure" LPAREN value COMMA value COMMA value COMMA value RPAREN  // - AllocationFailure(allocator: Allocator, layout: Layout, pointer: Pointer, reason: AllocationFailureReason): Records that an allocator returned a null pointer for a given layout and the associated failure reason.
primary_implementstrait_5: "ImplementsTrait" LPAREN value COMMA value RPAREN  // - ImplementsTrait(allocator: Allocator, trait: AllocatorTrait): An allocator implements a specific trait, indicating it provides the required interface.
primary_legaltraitimplementation_6: "LegalTraitImplementation" LPAREN value COMMA value COMMA value COMMA value RPAREN  // - LegalTraitImplementation(allocator: Allocator, trait: AllocatorTrait, underlying: NativeAllocator, policy: ExhaustionPolicy): A trait implementation is considered legal if the allocator implements the trait, wraps a native allocator with an abort-on-exhaustion policy.
primary_deallocatesmemory_7: "DeallocatesMemory" LPAREN value COMMA value COMMA value COMMA value RPAREN  // - DeallocatesMemory(allocator: Allocator, ptr: Pointer, layout: Layout, memory: Memory): An allocator deallocates the memory block identified by the given pointer and layout.
primary_callerguaranteesdeallocatable_8: "CallerGuaranteesDeallocatable" LPAREN value COMMA value RPAREN  // - CallerGuaranteesDeallocatable(ptr: Pointer, layout: Layout): A composite predicate expressing that the caller has satisfied all necessary pre-conditions for a safe call to `dealloc`: non-null pointer, valid allocation, matching layout, and no prior deallocation.
primary_allocatedbyallocator_9: "AllocatedByAllocator" LPAREN value COMMA value RPAREN  // - AllocatedByAllocator(ptr: Pointer, allocator: Allocator): Indicates that the pointer `ptr` refers to a memory block that was allocated by the specified `allocator` and that the block is still allocated (i.e., not yet deallocated). This predicate captures the core logic of the sentence, connecting the pointer to its owning allocator.
primary_memoryblockdeallocated_10: "MemoryBlockDeallocated" LPAREN value RPAREN  // - MemoryBlockDeallocated(memory: Memory): Indicates that a specific memory block has been deallocated by a dealloc call.
primary_mayresultinundefinedbehaviorondealloc_11: "MayResultInUndefinedBehaviorOnDealloc" LPAREN value COMMA value COMMA value COMMA value RPAREN  // - MayResultInUndefinedBehaviorOnDealloc(allocator: Allocator, ptr: Pointer, layout: Layout, behavior: UndefinedBehavior): Expresses that attempting to deallocate memory with a given allocator, pointer, and layout may lead to undefined behaviour when the caller does not guarantee the pre-conditions required for a safe deallocation.
primary_alloczeroedmayresultinundefinedbehavior_12: "AllocZeroedMayResultInUndefinedBehavior" LPAREN value COMMA value COMMA value RPAREN  // - AllocZeroedMayResultInUndefinedBehavior(allocator: Allocator, layout: Layout, behavior: UndefinedBehavior): The allocator's `alloc_zeroed` method may result in undefined behavior when given a layout, particularly when the layout is zero-sized.
primary_alloczeroedreturnsinitialized_13: "AllocZeroedReturnsInitialized" LPAREN value COMMA value COMMA value RPAREN  // - AllocZeroedReturnsInitialized(allocator: Allocator, layout: Layout, pointer: Pointer): Indicates that the allocator's `alloc_zeroed` method returns a pointer to a memory block that is guaranteed to be initialized.
primary_resizesmemoryblock_14: "ResizesMemoryBlock" LPAREN value COMMA value COMMA value RPAREN  // - ResizesMemoryBlock(old_memory: Memory, new_memory: Memory, new_size: Size): Indicates that a reallocation changes the size of a memory block to a specified new size, producing a new memory block.
primary_mayresultinundefinedbehavioronpointeraccess_15: "MayResultInUndefinedBehaviorOnPointerAccess" LPAREN value COMMA value COMMA value RPAREN  // - MayResultInUndefinedBehaviorOnPointerAccess(allocator: Allocator, ptr: Pointer, behavior: UndefinedBehavior): Expresses that any access to the specified pointer after realloc may result in undefined behaviour.
primary_callersatisfiesreallocrequirements_16: "CallerSatisfiesReallocRequirements" LPAREN value COMMA value COMMA value COMMA value RPAREN  // - CallerSatisfiesReallocRequirements(allocator: Allocator, ptr: Pointer, layout: Layout, new_size: Size): Indicates that the caller has satisfied all necessary preconditions for a safe call to the unsafe `realloc` method, including that the pointer is non-null, refers to a currently allocated memory block, matches the layout used in the original allocation, and that the new size is appropriately handled.
primary_newsizeispositive_17: "NewSizeIsPositive" LPAREN value RPAREN  // - NewSizeIsPositive(new_size: Size): Primary predicate stating that the `new_size` argument of a `realloc` call is strictly greater than zero.
primary_roundupsizetoalignment_18: "RoundUpSizeToAlignment" LPAREN value COMMA value COMMA value RPAREN  // - RoundUpSizeToAlignment(layout: Layout, size: Size, rounded: RoundedSize): Relates a `Layout`, an original `Size` (`new_size`), and the rounded size (`rounded`) obtained by rounding up to the nearest multiple of the layout's alignment.
primary_mayresultinundefinedbehavioronrealloc_19: "MayResultInUndefinedBehaviorOnRealloc" LPAREN value COMMA value COMMA value COMMA value COMMA value RPAREN  // - MayResultInUndefinedBehaviorOnRealloc(allocator: Allocator, ptr: Pointer, layout: Layout, new_size: Size, behavior: UndefinedBehavior): Expresses that attempting to call realloc with a given allocator, pointer, layout, and new size may lead to undefined behavior when preconditions are violated.
primary_allocatorcanallocate_20: "AllocatorCanAllocate" LPAREN value COMMA value RPAREN  // - AllocatorCanAllocate(allocator: Allocator, layout: Layout): Indicates that a given allocator is able to allocate a memory block that satisfies the size and alignment constraints of the specified layout.

?cond_atom: cond_pointerpointsto_0 | cond_isnullpointer_1 | cond_layoutsize_2 | cond_zerosizelayout_3 | cond_failurereasonismemoryexhaustion_4 | cond_failurereasonisconstraintviolation_5 | cond_constraintviolationreasonissizeconstraint_6 | cond_constraintviolationreasonisalignmentconstraint_7 | cond_wrapsnativeallocator_8 | cond_nativeallocatorhasexhaustionpolicy_9 | cond_exhaustionpolicyaborts_10 | cond_declaresunsafefunction_11 | cond_isvalidpointer_12 | cond_allocationrecordmatches_13 | cond_callerensurespointerisnonnull_14 | cond_callerensurespointerisvalid_15 | cond_callerensureslayoutmatchesallocation_16 | cond_callerensuresnodoublefree_17 | cond_allocatedmemoryblockofallocator_18 | cond_layoutmatchesmemory_19 | cond_pointerinvalidatedbydealloc_20 | cond_callerensuresnonzerolayout_21 | cond_memoryisinitialized_22 | cond_shrinksmemoryblock_23 | cond_growsmemoryblock_24 | cond_reallocinvalidatesoldpointer_25 | cond_updatedsize_26 | cond_minsize_27 | cond_rangevaluesequal_28 | cond_ownershipstatusforpointer_29 | cond_memoryblockcontentstatusforpointer_30 | cond_callerensuresnewsizeisnonzero_31 | cond_layoutmatchesallocation_32 | cond_sizeisnonzero_33 | cond_sizegreaterthanzero_34 | cond_roundedsizewithinisizemax_35 | cond_sizewithinisizemax_36 | cond_reallocpreconditionviolated_37 | cond_reallocfailurereasonisconstraintviolation_38 | cond_reallocfailurereasonissizeconstraintviolation_39 | cond_reallocfailurereasonisalignmentconstraintviolation_40

cond_pointerpointsto_0: "PointerPointsTo" LPAREN value COMMA value RPAREN  // - PointerPointsTo(pointer: Pointer, memory: Memory): A pointer refers to (points to) a specific memory region.
cond_isnullpointer_1: "IsNullPointer" LPAREN value RPAREN  // - IsNullPointer(pointer: Pointer): Indicates that a given pointer value is the null pointer used to signal allocation failure.
cond_layoutsize_2: "LayoutSize" LPAREN value COMMA value RPAREN  // - LayoutSize(layout: Layout, size: NonZeroSize): Relates a Layout to its size, which must be a non-zero value.
cond_zerosizelayout_3: "ZeroSizeLayout" LPAREN value RPAREN  // - ZeroSizeLayout(layout: Layout): Indicates that a layout specifies a size of exactly zero bytes.
cond_failurereasonismemoryexhaustion_4: "FailureReasonIsMemoryExhaustion" LPAREN value RPAREN  // - FailureReasonIsMemoryExhaustion(reason: AllocationFailureReason): Indicates that a given allocation failure reason is due to memory exhaustion.
cond_failurereasonisconstraintviolation_5: "FailureReasonIsConstraintViolation" LPAREN value RPAREN  // - FailureReasonIsConstraintViolation(reason: AllocationFailureReason): Indicates that a given allocation failure reason is due to a violation of the allocator's size or alignment constraints.
cond_constraintviolationreasonissizeconstraint_6: "ConstraintViolationReasonIsSizeConstraint" LPAREN value RPAREN  // - ConstraintViolationReasonIsSizeConstraint(reason: ConstraintViolationReason): Specifies that a constraint violation reason refers to a size constraint violation.
cond_constraintviolationreasonisalignmentconstraint_7: "ConstraintViolationReasonIsAlignmentConstraint" LPAREN value RPAREN  // - ConstraintViolationReasonIsAlignmentConstraint(reason: ConstraintViolationReason): Specifies that a constraint violation reason refers to an alignment constraint violation.
cond_wrapsnativeallocator_8: "WrapsNativeAllocator" LPAREN value COMMA value RPAREN  // - WrapsNativeAllocator(allocator: Allocator, underlying: NativeAllocator): An allocator is implemented atop an underlying native allocation library.
cond_nativeallocatorhasexhaustionpolicy_9: "NativeAllocatorHasExhaustionPolicy" LPAREN value COMMA value RPAREN  // - NativeAllocatorHasExhaustionPolicy(underlying: NativeAllocator, policy: ExhaustionPolicy): The underlying native allocator is configured with a specific exhaustion policy.
cond_exhaustionpolicyaborts_10: "ExhaustionPolicyAborts" LPAREN value RPAREN  // - ExhaustionPolicyAborts(policy: ExhaustionPolicy): A particular exhaustion policy causes the program to abort when memory is exhausted.
cond_declaresunsafefunction_11: "DeclaresUnsafeFunction" LPAREN value COMMA value RPAREN  // - DeclaresUnsafeFunction(allocator: Allocator, function: UnsafeFunction): The allocator declares an unsafe function as part of its interface.
cond_isvalidpointer_12: "IsValidPointer" LPAREN value RPAREN  // - IsValidPointer(ptr: Pointer): Indicates that the given pointer refers to a currently allocated (non-deallocated) memory block.
cond_allocationrecordmatches_13: "AllocationRecordMatches" LPAREN value COMMA value COMMA value RPAREN  // - AllocationRecordMatches(ptr: Pointer, layout: Layout, memory: Memory): Relates a pointer, layout and the memory block that was previously allocated for that pointer and layout.
cond_callerensurespointerisnonnull_14: "CallerEnsuresPointerIsNonNull" LPAREN value RPAREN  // - CallerEnsuresPointerIsNonNull(ptr: Pointer): Indicates that the pointer argument supplied to `dealloc` is not the null pointer, thereby avoiding the null-pointer edge case.
cond_callerensurespointerisvalid_15: "CallerEnsuresPointerIsValid" LPAREN value RPAREN  // - CallerEnsuresPointerIsValid(ptr: Pointer): Indicates that the pointer argument refers to a currently allocated (non-deallocated) memory block.
cond_callerensureslayoutmatchesallocation_16: "CallerEnsuresLayoutMatchesAllocation" LPAREN value COMMA value RPAREN  // - CallerEnsuresLayoutMatchesAllocation(ptr: Pointer, layout: Layout): Indicates that the layout argument supplied to `dealloc` exactly matches the layout that was used during the original allocation of the pointer.
cond_callerensuresnodoublefree_17: "CallerEnsuresNoDoubleFree" LPAREN value RPAREN  // - CallerEnsuresNoDoubleFree(ptr: Pointer): Indicates that the pointer has not already been freed by a prior call to `dealloc`, preventing double free.
cond_allocatedmemoryblockofallocator_18: "AllocatedMemoryBlockOfAllocator" LPAREN value COMMA value RPAREN  // - AllocatedMemoryBlockOfAllocator(memory: Memory, allocator: Allocator): Associates a memory block with the allocator that performed the allocation. This predicate allows other rules (e.g., deallocation) to verify that the deallocating allocator matches the allocating allocator.
cond_layoutmatchesmemory_19: "LayoutMatchesMemory" LPAREN value COMMA value RPAREN  // - LayoutMatchesMemory(layout: Layout, memory: Memory): Indicates that a given layout was used to allocate a specific memory block.
cond_pointerinvalidatedbydealloc_20: "PointerInvalidatedByDealloc" LPAREN value COMMA value RPAREN  // - PointerInvalidatedByDealloc(ptr: Pointer, allocator: Allocator): Denotes that a pointer, after a successful dealloc call, no longer refers to a valid allocated memory block.
cond_callerensuresnonzerolayout_21: "CallerEnsuresNonZeroLayout" LPAREN value RPAREN  // - CallerEnsuresNonZeroLayout(layout: Layout): Indicates that the caller provides a layout whose size component is strictly greater than zero, ensuring the layout is non-zero.
cond_memoryisinitialized_22: "MemoryIsInitialized" LPAREN value RPAREN  // - MemoryIsInitialized(memory: Memory): Denotes that a memory block is initialized.
cond_shrinksmemoryblock_23: "ShrinksMemoryBlock" LPAREN value COMMA value COMMA value RPAREN  // - ShrinksMemoryBlock(old_memory: Memory, new_memory: Memory, new_size: Size): Specifies that the reallocation results in a memory block whose new size is strictly smaller than the original block's size.
cond_growsmemoryblock_24: "GrowsMemoryBlock" LPAREN value COMMA value COMMA value RPAREN  // - GrowsMemoryBlock(old_memory: Memory, new_memory: Memory, new_size: Size): Specifies that the reallocation results in a memory block whose new size is strictly larger than the original block's size.
cond_reallocinvalidatesoldpointer_25: "ReallocInvalidatesOldPointer" LPAREN value COMMA value RPAREN  // - ReallocInvalidatesOldPointer(allocator: Allocator, old_ptr: Pointer): Indicates that the old pointer is invalidated by a realloc call on the given allocator.
cond_updatedsize_26: "UpdatedSize" LPAREN value COMMA value COMMA value RPAREN  // - UpdatedSize(old_layout: Layout, new_size: Size, new_layout: Layout): Indicates that a new layout is derived from an existing layout by updating its size component to a specified new size.
cond_minsize_27: "MinSize" LPAREN value COMMA value COMMA value RPAREN  // - MinSize(layout: Layout, new_size: Size, min: Size): Relates a Layout, a requested new size, and the minimum of their sizes.
cond_rangevaluesequal_28: "RangeValuesEqual" LPAREN value COMMA value COMMA value RPAREN  // - RangeValuesEqual(old_memory: Memory, new_memory: Memory, length: Size): Expresses that two memory blocks have identical byte values for all offsets less than a given length.
cond_ownershipstatusforpointer_29: "OwnershipStatusForPointer" LPAREN value COMMA value RPAREN  // - OwnershipStatusForPointer(ptr: Pointer, status: OwnershipStatus): Links a pointer to its ownership status after a realloc call. The status indicates whether the allocator has transferred ownership of the memory block to the caller.
cond_memoryblockcontentstatusforpointer_30: "MemoryBlockContentStatusForPointer" LPAREN value COMMA value RPAREN  // - MemoryBlockContentStatusForPointer(ptr: Pointer, status: MemoryBlockContentStatus): Links a pointer to the content status of the memory block it refers to after a realloc call. The status indicates whether the contents of the memory block have been altered or remain unaltered.
cond_callerensuresnewsizeisnonzero_31: "CallerEnsuresNewSizeIsNonZero" LPAREN value RPAREN  // - CallerEnsuresNewSizeIsNonZero(new_size: Size): Indicates that the new size argument supplied to `realloc` is strictly greater than zero, which is a common requirement for non-zero reallocations. (The zero-size case is handled separately by the `ZeroSizeRealloc` rule.)
cond_layoutmatchesallocation_32: "LayoutMatchesAllocation" LPAREN value COMMA value RPAREN  // - LayoutMatchesAllocation(ptr: Pointer, layout: Layout): Indicates that the layout argument passed to `realloc` is the same layout that was used to allocate the memory block referenced by the pointer.
cond_sizeisnonzero_33: "SizeIsNonZero" LPAREN value RPAREN  // - SizeIsNonZero(size: Size): Normal predicate relating an arbitrary size value to the `NonZeroSize` sort, indicating that the size is strictly greater than zero.
cond_sizegreaterthanzero_34: "SizeGreaterThanZero" LPAREN value RPAREN  // - SizeGreaterThanZero(size: Size): Normal predicate expressing the basic numeric property that a size value is greater than zero.
cond_roundedsizewithinisizemax_35: "RoundedSizeWithinIsizeMax" LPAREN value COMMA value RPAREN  // - RoundedSizeWithinIsizeMax(layout: Layout, size: Size): Specifies that the rounded size computed from a `Layout` and `Size` does not overflow `isize` (i.e., the rounded value is less than or equal to `isize::MAX`).
cond_sizewithinisizemax_36: "SizeWithinIsizeMax" LPAREN value RPAREN  // - SizeWithinIsizeMax(size: Size): Expresses that a given `Size` value is less than or equal to `isize::MAX`.
cond_reallocpreconditionviolated_37: "ReallocPreconditionViolated" LPAREN value COMMA value COMMA value COMMA value RPAREN  // - ReallocPreconditionViolated(allocator: Allocator, ptr: Pointer, layout: Layout, new_size: Size): Indicates that the caller has violated one or more preconditions required before calling the unsafe realloc method, such as passing a null or invalid pointer, mismatched layout, or improper new size.
cond_reallocfailurereasonisconstraintviolation_38: "ReallocFailureReasonIsConstraintViolation" LPAREN value RPAREN  // - ReallocFailureReasonIsConstraintViolation(reason: ReallocFailureReason): Denotes that a reallocation failure reason is due to a violation of the allocator's size or alignment constraints.
cond_reallocfailurereasonissizeconstraintviolation_39: "ReallocFailureReasonIsSizeConstraintViolation" LPAREN value RPAREN  // - ReallocFailureReasonIsSizeConstraintViolation(reason: ReallocFailureReason): Specifies that the reallocation failure reason is caused by a size constraint violation.
cond_reallocfailurereasonisalignmentconstraintviolation_40: "ReallocFailureReasonIsAlignmentConstraintViolation" LPAREN value RPAREN  // - ReallocFailureReasonIsAlignmentConstraintViolation(reason: ReallocFailureReason): Specifies that the reallocation failure reason is caused by an alignment constraint violation.
```

Natural-language rule:```
`ptr` is a block of memory currently allocated via this allocator and,
```

Associated Target:```
unsafe fn dealloc(&self, ptr: *mut u8, layout: Layout);
```

Target Attributes in JSON format:```
{
    "name": "dealloc",
    "safety": "unsafe",
    "kind": "fn",
    "parameters": [
      {
        "name": "self",
        "type": "&Self"
      },
      {
        "name": "ptr",
        "type": "*mut u8"
      },
      {
        "name": "layout",
        "type": "Layout"
      }
    ],
    "receiver_type": "&Self",
    "receiver_mutability": false,
    "is_method": true,
    "receiver_name": "self",
    "parameter_count": 2,
    "function_has_body": false
}
```
Analyze the request step by step, then respond with JSON in the following format
{{
    "analysis": "Your analysis here",
    "actions": [
        {{
            "name": "action_name",
            "input": {{
                // action input according to the schema
            }}
        }}
    ]
}}
\end{lstlisting}
\end{llmex}

\vspace{6pt}

\begin{llmex}{LLM Output (Response)}
\begin{lstlisting}[style=llmtext]
{
  "analysis": "The natural-language rule states that `ptr` refers to a memory block that is currently allocated by this allocator. The corresponding predicate is `AllocatedByAllocator(ptr, self)`. Thus the full statement is `AllocatedByAllocator(ptr, self)`.",
  "actions": [
    {
      "name": "write_dsl",
      "input": {
        "dsl": "AllocatedByAllocator(ptr, self);"
      }
    }
  ]
}
\end{lstlisting}
\end{llmex}
