# Supplementary material for: Doc2Spec: Synthesizing Formal Programming Specifications from Natural Language via Grammar Induction
Source: arXiv:2602.04892 source file (2026-10-07)
Supplement: Supplementary file 2 [file 01_entity_scope_discovery.response.tex]

% Generated by scripts/render_response_views.py; edit the renderer, not this file.
\ResponseField{Entity patterns}{None (empty list).}
\ResponseField{Scope patterns}{None (empty list).}
