# Supplementary material for: Doc2Spec: Synthesizing Formal Programming Specifications from Natural Language via Grammar Induction
Source: arXiv:2602.04892 source file (2026-10-07)
Supplement: Supplementary file 3 [file 02_entity_entity_discovery.response.tex]

% Generated by scripts/render_response_views.py; edit the renderer, not this file.
\ResponseGroup{Entity patterns: 1}
\ResponseField{Kind}{\texttt{function}}
\ResponseField{Start regex}{\texttt{\textasciicircum{}function\textbackslash{}s+[A-Za-z\_][A-Za-z0-9\_]*\textbackslash{}b}}
\ResponseField{Example}{\texttt{function transferFrom(address \_from, address \_to, uint256 \_value) public returns (bool success)}}
\ResponseField{Scope patterns}{None (empty list).}
