# Supplementary material for: Doc2Spec: Synthesizing Formal Programming Specifications from Natural Language via Grammar Induction
Source: arXiv:2602.04892 source file (2026-10-07)
Supplement: Supplementary file 4 [file 03_entity_pattern_validation.response.tex]

% Generated by scripts/render_response_views.py; edit the renderer, not this file.
\ResponseGroup{entity-pattern-0001}
\ResponseField{Keep pattern}{\texttt{true}}
\ResponseField{Rationale}{Matches a Solidity function declaration, which is a valid entity definition for attaching behavioral documentation.}
