# Supplementary material for: Doc2Spec: Synthesizing Formal Programming Specifications from Natural Language via Grammar Induction
Source: arXiv:2602.04892 source file (2026-10-07)
Supplement: Supplementary file 5 [file 04_entity_candidate_classification.response.tex]

% Generated by scripts/render_response_views.py; edit the renderer, not this file.
\ResponseGroup{candidate-0001}
\ResponseField{Entity}{\texttt{true}}
\ResponseField{Declaration end line}{7}
\ResponseField{Enclosing scopes}{None (empty list).}
\ResponseField{Kind}{\texttt{function}}
\ResponseField{Name}{\texttt{transferFrom}}
\ResponseField{Visibility}{\texttt{public}}
\ResponseGroup{Parameters (declaration order)}
\begin{tabularx}{\linewidth}{@{}lXX@{}}
\toprule
\textbf{Position} & \textbf{Name} & \textbf{Type} \\
\midrule
1 & \texttt{\_from} & \texttt{address} \\
2 & \texttt{\_to} & \texttt{address} \\
3 & \texttt{\_value} & \texttt{uint256} \\
\bottomrule
\end{tabularx}\par
\ResponseGroup{Return values (declaration order)}
\begin{tabularx}{\linewidth}{@{}lXX@{}}
\toprule
\textbf{Position} & \textbf{Name} & \textbf{Type} \\
\midrule
1 & \texttt{success} & \texttt{bool} \\
\bottomrule
\end{tabularx}\par
