# Supplementary material for: Doc2Spec: Synthesizing Formal Programming Specifications from Natural Language via Grammar Induction
Source: arXiv:2602.04892 source file (2026-10-07)
Supplement: Supplementary file 6 [file 05_rule_clause_extraction.response.tex]

% Generated by scripts/render_response_views.py; edit the renderer, not this file.
\ResponseGroup{Clause 1}
Transfers \_value amount of tokens from address \_from to address \_to, and MUST fire the Transfer event.\par
\ResponseGroup{Clause 2}
Transfers of 0 values MUST be treated as normal transfers and fire the Transfer event.\par
\ResponseGroup{Clause 3}
The function SHOULD throw unless the \_from account has deliberately authorized the sender of the message via some mechanism.\par
