# Supplementary material for: Doc2Spec: Synthesizing Formal Programming Specifications from Natural Language via Grammar Induction
Source: arXiv:2602.04892 source file (2026-10-07)
Supplement: Supplementary file 7 [file 06_rule_candidate_scoring.response.tex]

% Generated by scripts/render_response_views.py; edit the renderer, not this file.
\begin{tabularx}{\linewidth}{@{}Xll@{}}
\toprule
\textbf{Candidate} & \textbf{Rule label} & \textbf{Confidence} \\
\midrule
\texttt{candidate-0003} & \texttt{true} & 0.8 \\
\bottomrule
\end{tabularx}\par
\ResponseGroup{candidate-0003: rationale}
Specifies a behavioral expectation (the function should throw when unauthorized), which can be tested; although not a MUST, it is still a non-vague, enforceable rule.\par
