# Supplementary material for: Doc2Spec: Synthesizing Formal Programming Specifications from Natural Language via Grammar Induction
Source: arXiv:2602.04892 source file (2026-10-07)
Supplement: Supplementary file 8 [file 07_predicate_semantic_analysis.response.tex]

% Generated by scripts/render_response_views.py; edit the renderer, not this file.
\ResponseGroup{C\_authorized}
\ResponseField{Role}{condition}
\ResponseField{Source span}{the \_from account has deliberately authorized the sender of the message via some mechanism}
\ResponseField{Meaning}{The \_from account has deliberately authorized the message sender via some mechanism}
\ResponseField{Parameters (in order)}{\texttt{\_from}, \texttt{sender}}
\ResponseGroup{O\_throw}
\ResponseField{Role}{obligation}
\ResponseField{Source span}{throw}
\ResponseField{Meaning}{The function reverts execution}
\ResponseField{Parameters (in order)}{None (empty list).}
\ResponseGroup{Boolean structure}
\ResponseField{Outcome formula}{\texttt{O\_throw}}
\ResponseField{Condition formula}{\texttt{not C\_authorized}}
