# Supplementary material for: Doc2Spec: Synthesizing Formal Programming Specifications from Natural Language via Grammar Induction
Source: arXiv:2602.04892 source file (2026-10-07)
Supplement: Supplementary file 9 [file 08_predicate_vocabulary_synthesis.response.tex]

% Generated by scripts/render_response_views.py; edit the renderer, not this file.
\ResponseGroup{Sorts}
\ResponseField{Address}{Ethereum address}
\ResponseGroup{Predicate: AuthorizedCondition}
\ResponseField{Source atom}{\texttt{C\_authorized}}
\ResponseField{Signature}{\texttt{AuthorizedCondition(\_from: Address, sender: Address)}}
\ResponseField{Meaning}{The \_from account has deliberately authorized the message sender via some mechanism}
\ResponseGroup{Predicate: ThrowObligation}
\ResponseField{Source atom}{\texttt{O\_throw}}
\ResponseField{Signature}{\texttt{ThrowObligation()}}
\ResponseField{Meaning}{The function reverts execution}
