# Supplementary material for: Doc2Spec: Synthesizing Formal Programming Specifications from Natural Language via Grammar Induction
Source: arXiv:2602.04892 source file (2026-10-07)
Supplement: Supplementary file 10 [file 09_formalize_dsl_translation.response.tex]

% Generated by scripts/render_response_views.py; edit the renderer, not this file.
\ResponseField{DSL statement}{\texttt{SHOULD ThrowObligation() if not AuthorizedCondition(\_from, sender);}}
