# Supplementary material for: Doc2Spec: Synthesizing Formal Programming Specifications from Natural Language via Grammar Induction
Source: arXiv:2602.04892 source file (2026-10-07)
Supplement: Supplementary file 11 [file erc721_scope.response.tex]

% Generated by scripts/render_response_views.py; edit the renderer, not this file.
\ResponseGroup{Scope patterns: 1}
\ResponseField{Kind}{\texttt{interface}}
\ResponseField{Start regex}{\texttt{\textasciicircum{}interface\textbackslash{}s+(?P<name>\textbackslash{}w+)\textbackslash{}b.*\textbackslash{}\{}}
\ResponseField{Example}{\texttt{interface ERC721Metadata /* is ERC721 */ \{}}
\ResponseField{Opening regex}{\texttt{\textbackslash{}\{}}
\ResponseField{Closing regex}{\texttt{\textbackslash{}\}}}
\ResponseField{Role}{\texttt{semantic\_container}}
