# Supplementary material for: Doc2Spec: Synthesizing Formal Programming Specifications from Natural Language via Grammar Induction
Source: arXiv:2602.04892 source file (2026-10-07)
Supplement: Supplementary file 12 [file resolve_ebnf_error.tex]

\begin{llmex}{Prompt Template}
\begin{lstlisting}[style=llmtext]
You can perform the following actions.
Available Actions:
- write_dsl: Return exactly one DSL statement that conforms to the provided grammar for the given rule.
  Input Schema: {
  "type": "object",
  "properties": {
    "dsl": {
      "type": "string",
      "description": "A single DSL statement that ends with ';' and parses with the grammar."
    }
  },
  "required": [
    "dsl"
  ]
}


Write ONE DSL statement for the given natural-language rule, using the following Lark grammar.
Rules:
- The DSL must parse with this grammar.
- Do NOT invent predicate names or change arity; only use what appears in the grammar.
- Output exactly one statement and end it with ';'.
- If rule requires certain attributes from the target(provided in JSON format), use JSON path to access them.

Grammar:```
(*@\hlline{0.11}@*){{grammar}}
```

Natural-language rule:```
(*@\hlline{0.11}@*){{sentence}}
```


Associated Target:```
(*@\hlline{0.10}@*){{entity}}
```

Target Attributes in JSON format:```
(*@\hlline{0.20}@*){{entity_attributes}}
```

Previous attempt and error (fix it): (*@\hlline{0.16}@*){{dsl}} {{error}}

Analyze the request step by step, then respond with JSON in the following format
{
    "analysis": "Your analysis here",
    "actions": [
        {
            "name": "action_name",
            "input": {
                // action input according to the schema
            }
        }
    ]
}
\end{lstlisting}
\end{llmex}
