# Supplementary material for: Doc2Spec: Synthesizing Formal Programming Specifications from Natural Language via Grammar Induction
Source: arXiv:2602.04892 source file (2026-10-07)
Supplement: Supplementary file 13 [file resolve_json_error.tex]

\begin{llmex}{Prompt Template}
\begin{lstlisting}[style=llmtext]
Last Response:```
(*@\hlline{0.20}@*){{previous_response}}
```
There was an error processing the last response:```
(*@\hlline{0.09}@*){{error}}
``` 
Please refine your last response to fix the error.
Respond with JSON only, without any additional text.
\end{lstlisting}
\end{llmex}
