# Supplementary material for: Doc2Spec: Synthesizing Formal Programming Specifications from Natural Language via Grammar Induction
Source: arXiv:2602.04892 source file (2026-10-07)
Supplement: Supplementary file 14 [file resolve_regex_error.tex]

\begin{llmex}{Prompt Template}
\begin{lstlisting}[style=llmtext]
Regex Pattern:```
(*@\hlline{0.11}@*){{pattern}}
```
Example to be matched:```
(*@\hlline{0.11}@*){{example}}
```
Error Message:```
(*@\hlline{0.09}@*){{error}}
```
Please provide a corrected regex pattern that resolves the error.
\end{lstlisting}
\end{llmex}
