# Supplementary material for: Doc2Spec: Synthesizing Formal Programming Specifications from Natural Language via Grammar Induction
Source: arXiv:2602.04892 source file (2026-10-07)
Supplement: Supplementary file 15 [file resolve_schema_err.tex]

\begin{llmex}{Prompt Template}
\begin{lstlisting}[style=llmtext]
Data:```
(*@\hlline{0.26}@*){{previous_responsed_json}}
```
Schema:```
(*@\hlline{0.19}@*){{expected_schema}}
```
There was an error validating the data against the schema:```
(*@\hlline{0.09}@*){{error}}
```
Please refine the data to conform to the schema.
Respond with JSON only, without any additional text.
\end{lstlisting}
\end{llmex}
